# Supplementary material for: The Devil is in the Details: On Models and Training Regimes for Few-Shot Intent Classification
Source: arXiv:2210.06440 source file (2022-10-12)
Supplement: Supplementary file 1 [file appendix.tex]

\section{Data Statistics}

\begin{table*}[!t]
    %\small
    \centering
    \begin{tabular}{@{}l@{}rrrcrrcrrr@{}}
        \toprule 
                
                & \multicolumn{3}{c}{\textbf{ATIS}} && \multicolumn{2}{c}{\textbf{SNIPS}} && \multicolumn{3}{c}{\textbf{TOP}} \\        
         \cmidrule{2-4}\cmidrule{6-7}\cmidrule{9-11}
                & Train & Dev & Test && Train &  Test && Train & Dev & Test  \\
         \midrule
             \# Sent.  &  4,373 & 662 & 829 &&   8,230 &  6,254 && 20,345 & 4,333 & 4,426 \\
             \# Intents & 5 & 7 & 7 && 4  &  3 &&  7 & 5 & 6\\
             \# Episodes  & 1,377	&213	&119 && 240 & 210 && 10,095 & 1,286 &	292 \\
             \midrule
             \textit{Per episode} \\
             \hspace{1ex}Avg. \# intents&  4	 &	5 &		5	 &&	3.5	 &		3	&&		5	 &	4 &		4.5 \\
             \hspace{1ex}Avg. |sup.|  & 15.54	&  16.77	& 17.08	&&  17.28	&  16.56	&& 15.81	& 16.16& 17.24 \\
             \hspace{1ex}(Min, Max)  |sup.|  & (8, 19) &	(11, 19) &	(12, 19) &&			(16, 19) &		(16, 17) &&	(3, 19) &	(9, 19)	 &(16, 19) \\
             %\hspace{2ex} min.  sup. size & 8 &	11 &	12 &&			16 &		16 &&	3 &	9	 &16 \\
             %\hspace{2ex}max.  sup. size &  19	 &	19	 &	19 &&		19	 &		17	 &&		19	 &	19	 &	 19 \\
             \hspace{1ex}Avg. |query|  & 14.52 	& 	14.65	& 	14.91	&& 	35.08		& 	30		&&  6.16 	& 7.9	& 45.31 \\
             \hspace{1ex}(Min, Max) |query|  & (9, 30) & (3, 60) &	(3, 60)	&& (30, 40)	&	(30, 30)	&&	(3,40) &	(3, 40)	& (30,60) \\
            %\hspace{2ex}min. query size & 9 & 3 &	3	&&30	&	30	&&	3 &	3	& 30 \\
             %\hspace{2ex}max. query size  & 30 &	60 & 60	&&	40	&	30	&&	40&	30&	60 \\
        \bottomrule
    \end{tabular}
    \caption{\textbf{Dataset properties.} 
    The statistics of the few-shot learning splits constructed for each corpus. 
    ``|sup.|'' and ``|query|'' indicate the size or the number of examples in support sets and query sets, respectively. 
    ``Avg.'' stands for average.  }
    \label{tab:datasets}
\end{table*}
